# Supplementary material for: Putting Things into Context: Rich Explanations for Query Answers using Join Graphs (extended version)
Source: arXiv:2103.15797 source file (2021-03-29)
Supplement: Supplementary file 1 [file appendix.tex]

\section{appendix}
\begin{example}
\label{eg:running}
Consider a simplified version of our \nbadata dataset  with the tables shown in \Cref{fig:running-base}
\begin{itemize}
    % \item {\tt PlayFor(\underline{player, team, start\_year, start\_month}, \\ \underline{start\_day}, end\_year, end\_month, end\_day)} contains the information about when did a player play for an NBA team.
\item {\tt PlayerGameScoring(\underline{player, year, month, day}, home, mp, pts)} contains the statistics about scoring (minutes played, points for every player in every game.
% \item {\tt LineupTeam(\underline{lineupid, team})} contains the lineups of all teams.
\item {\tt LineupPlayer(\underline{lineupid, player})} contains the players in all lineups.
\item {\tt LineupPerGameStats(\underline{lineupid, year, month, day}, mp, poss,  pace)} contains the statistics about minutes played, the number of offensive possessions, the estimated number of possessions per game for the certain lineup.
\item {\tt Game(\underline{year, month, day, home}, away, home\_pts, away\_pts, winner, season)} contains the information about participating teams and the winner in each NBA game.
% \item {\tt TeamGameAssist(\underline{year, month, day, team}, assists, \\assistpts, two\_ptassists, three\_ptassists)} contains the statistics about assists for each team in each NBA game.
% \item {\tt TeamGameScoring(\underline{year, month, day, team}, pts, fg\_two\_m, fg\_two\_a, fg\_two\_pct, fg\_three\_m, fg\_three\_a, fg\_three
% \_pct)} contains the statistics about scoring for each team in each NBA game.
% \item Tables {\tt Team(teamid, name)}, {\tt Season(seasonid, season\_name)}, and {\tt Player(playerid, player\_name)} contains information ...\red{please finish}
\end{itemize}

\cut{
\SR{The attribute and table names are not consistent -- to fix.

Can you put all the base table instances in a single figure* with (a) (b) (c) etc? They should match the schema in Ex 1.

I suggest to get rid of Team and Season table (also Player) in this simplified example, and use the names of teams, players, and seasons directly in the other tables -- these are one-one joins, are these tables useful in making a point?}
}

Figure~\ref{fig:running-base} shows a partial instance for the above schema. Suppose a user wants to see how the average points per game evolve in each month for all the players, and runs the following SQL query $Q_0$ that uses only the {\tt PlayerGameScoring} table.
%computes the average points per game for every player per month and uses only the {\tt PlayerGameScoring} table.

%\SR{use year and month columns in Table 1?}

\begin{lstlisting}
Q_0: SELECT player, year, month, avg(pts) AS avg_pts
     FROM PlayerGameScoring
     GROUP BY player, year, month
     ORDER BY player, year, month
\end{lstlisting}

%%%%%%%%%%%%%%%%%%%%%%%%%%%%%%%%%%%%%%%%

Figure~\ref{table:SB} shows a subset of this query's
result for player  \playerSB{} (Shane Battier). After querying the average points per month, a user may be interested in knowing why in certain months \playerSB{} scored much lower/higher compared to other months.
For instance,
\begin{tcolorbox}[colback=white,left=2pt,right=2pt,top=0pt,bottom=0pt]
$\uquestion_0$: {\bf ``why did \playerSB{} score only 2.20 per game in Jan 2013, which is much lower than 9.08 in Feb 2013?''}
\end{tcolorbox}

To answer such a question in the above example, we can look into the \emph{provenance} of these two result tuples, which would enumerate input tuples from the {\tt PlayerGameScoring} table that contributed to the query results $\egTup = $ \textsc{(\playerSB{}, 2013, 1, 2.20)} and \textsc{(\playerSB{}, 2013, 2, 9.08)}.
%, i.e., games that \playerSB{} played in Jan. 2013.
However, these tuples do not easily help us understand why the average points of \ \playerSB{} in Jan. 2013 is low. As a second attempt, we may look into additional summarization over these tuples in the {\tt PlayerGameScoring} table as follows:\\

{\scriptsize
\begin{tabular}{|cccccccc|} \hline
\rowcolor{grey} \textbf{player} & \textbf{year} & \textbf{month} & \textbf{avg\_mp} & \textbf{avg\_pts} & \textbf{avg\_fgm} & \textbf{avg\_fga} & \textbf{avg\_usg}   \\ \hline
%$\playerSB{}$ & 2012 & 11 & 26.34&   7.08&   2.33&   5.25&  11.89 \\
%$\playerSB{}$ & 2012 & 12 &  24.57&   6.46&   2.00&  5.38&  11.60\\
$\playerSB{}$ & {\bf 2013} & {\bf 1} &  20.95& {\bf2.20}&   0.70&   3.90&  10.72\\
$\playerSB{}$ & {\bf 2013} & {\bf 2} & 26.36& {\bf 9.08}&   3.00&   5.67&  11.63\\
%$\playerSB{}$ & 2013 & 3 & 24.77&   7.00&   2.28&   4.89&  10.97\\
\hline
\end{tabular}
}\\

This summarization does reveal the informative fact that \playerSB{} played less number of minutes on average in Jan 2013 compared to Feb 2013. However, the other statistics showing lower average field goals made/attempted and usage percentage of team plays merely reinforce the lower score in Jan 2013 and do not provide deeper insights `\emph{why}' the average score was lower in this month.
%on other statistics about \playerSB{}'s performance in these games (e.g., minutes played per game or field goals attempted per game) are neither informative nor interesting.
\end{example}

%\SR{Can you write in comments what the average values of the other fields are in this table?}
%\ZM{Put them in the comment below.}

\cut{
\SR{I am writing the full schema in the above example, otherwise it seems that we have not given the reader  full information on the database to think about possible solutions.}
}

Example~\ref{eg:running} raises the question that what if the tables used in the user query do not contain enough information to explain unexpected query results?
As we have seen in the example, to understand why a player performs poorly in a certain period, an explanation built only on the player's scoring records from the table used in the query ({\tt PlayerGameScoring} table) may not be enough, because these tables only contain information on scoring itself while there are other external factors affecting the game performance.
For example, lineups would have a strong impact on players' scoring efficiency, the strength/weakness of the opponents play a role, and the pace of the game can also largely affect players' points.

\begin{example}
\label{eg:running-lineup}
To show that how tables not used in the query can help provide explanations to the question in Example~\ref{eg:running}, let us consider two other tables in the NBA statistics dataset, \texttt{LineupPlayer} and \texttt{LineupPerGameStats} (see Figures~\ref{table:lp} and Figure~\ref{table:lpgs} for example tuples), which contain the information about the players in the lineups and the overall statistics of each lineup in every game. %Figure~\ref{table:lp} and Figure~\ref{table:lpgs} present example tuples in these two tables.
To see whether there is a player who had an impact on \playerSB{}'s average points, the user can join table \texttt{LineupPlayer} twice and \texttt{LineupPerGameStats} once with the table \textsc{PlayerGameScoring} in $Q_0$, to find players who played together with \playerSB{} during the time period in the user's question. Some tuples of the join result are presented in Table~\ref{table:running-example-SBlineup}. And one may find that in Jan. 2013, when \playerSB{} performed poorly, he played less time together with \playerLJ{} (Lebron James), which may explain the drop in his points per game.

\begin{tcolorbox}[colback=white,left=2pt,right=2pt,top=0pt,bottom=0pt]
% \playerSB{} only scored 2.20 per game in Jan. 2013 because Player: \playerLJ{}'s lineup minutes with him is more often (4/10) in the range of $ [0,12] $ compared to those in Feb. 2013 (1/12).
% \playerSB{} only scored 2.20 per game in Jan. 2013 because Player: \playerLJ{}'s lineup minutes with him is $<= 9.4$ in 4 out of 10 games compared to 0 out of 12 games in Feb. 2013.
\playerSB{} only scored 2.20 per game in Jan. 2013 because Player: \playerLJ{}'s lineup minutes with him is $ \geq 12$ in \underline{\bf 12 out of 12} games in Feb. 2013 compared with \underline{\bf 6 out of 10} games in Jan. 2013. %and 12>6
\end{tcolorbox}
%\SR{We need to say that we would discuss the scoring function later -- just saying $12>6$ might be confusing as the question of absolute number vs. fractions would arise.}
% \ZM{detailed explanation will be updated later} \SR{need the Feb 2013 info here too.}
\cut{
\ZM{If we consider directions when finding patterns, i.e., divide tuples in provenance into high/low groups, we may have some explanations likes these:}
}
% \begin{tcolorbox}[colback=white,left=2pt,right=2pt,top=0pt,bottom=0pt]
% \playerSB{} only scored 2.20 per game in Jan. 2013 because Player: \playerLJ{}'s lineup minutes with him is $<= 15.2$ in 5 out of 10 games with 1.0 precision on low-scoring ($<= avg(Jan + Feb) = 5.95$) compared to 3 out of 12 games in Feb. 2013.
% \playerSB{} only scored 2.20 per game in Jan. 2013 because Player: \playerLJ{}'s lineup minutes with him is $<= 9.4$ in 4 out of 9 low-scoring games (with precision 1.0) compared to 0 out of 3 low-scoring games ((with precision 0.0) in Feb. 2013.
% \end{tcolorbox}

% \begin{tcolorbox}[colback=white,left=2pt,right=2pt,top=0pt,bottom=0pt]
% \playerSB{} only scored 2.20 per game in Jan. 2013 because Player: \playerLJ{}'s lineup minutes with him is $<= 15.2$ in 5 out of 9 low-scoring ($<= avg(Jan+Feb) = 5.95$) games with 1.0 precision, compared to the range $>15.2$ in 8 out of 9 high-scoring ($> avg(Jan+Feb) = 5.95$) games with $8/9$ precision in Feb. 2013.
% \end{tcolorbox}

% Moreover, by considering the team statistics tables, the user may find that the defense quality of the opponents can also have an impact on \playerSB{}'s scoring. By joining tables \texttt{TeamGameScoring} and \texttt{Game}, the user obtains the information about the average opponents' three point field goals made of Miami's opponents.
Moreover, by considering a larger context and including the team statistics tables, the user may find that the number of team three-pointer assists is also related to \playerSB{}'s scoring. By joining table \texttt{LineupTeam} and \texttt{TeamGameAssist} with \texttt{PlayerGameScoring}, the user could find out that in Jan. 2013, Miami players assisted less three pointers compared to Feb. 2013, which can lead to the explanation that Miami might adjust its three-point strategies during these Jan. 2013 and thus it had an impact on \playerSB{}'s performance.

% \begin{tcolorbox}[colback=white,left=2pt,right=2pt,top=0pt,bottom=0pt]
% \playerSB{} only scored 2.20 per game in Jan. 2013 because the the team 3-pointer assists often in the range of $ [1,7] $ (6/10 games where \playerSB{} all scored poorly) compared to the range $[8,14]$ (6/12 games where \playerSB{} scored at least 12 points in 4/6 games) in Feb. 2013 .
% \playerSB{} only scored 2.20 per game in Jan. 2013 because the team 3-pointer assists is $<=7$ in 6 out of 9 low-scoring games ($<= 5.95$) with precision 1.0 compared to 3 out of 3 low-scoring games with precision 0.5 in Feb. 2013 .
% \end{tcolorbox}

\begin{tcolorbox}[colback=white,left=2pt,right=2pt,top=0pt,bottom=0pt]
% \playerSB{} only scored 2.20 per game in Jan. 2013 because the the team 3-pointer assists often in the range of $ [1,7] $ (6/10 games where \playerSB{} all scored poorly) compared to the range $[8,14]$ (6/12 games where \playerSB{} scored at least 12 points in 4/6 games) in Feb. 2013 .
% \playerSB{} only scored 2.20 per game in Jan. 2013 because the team 3-pointer assists is $<=7$ in 6 out of 9 low-scoring games ($<= 5.95$) with precision 1.0, compared to $>8$ in 6 out of 9 high-scoring games with precision 1.0 in Feb. 2013. While the range $>8$ is only in 1 out of 1 high-scoring games with precision $1/3$  in Jan. 2013.
\playerSB{} only scored 2.20 per game in Jan. 2013 because the team 3-pointer assists is $ \leq 8$ in \underline{\bf 10 out of 10} games in Jan. 2013 compared with \underline{\bf 7 out of 12} games in Feb. 2013. %and 10>7
\end{tcolorbox}
\end{example}

\begin{figure*}\scriptsize\setlength{\tabcolsep}{3pt}
\begin{minipage}{0.9\linewidth}\centering
    {\scriptsize
      \begin{tabular}{|ccccccccccccccc|} \hline
\rowcolor{grey} \textbf{game\_date} & \textbf{mp} & \textbf{pts} & \textbf{team\_pts} & \textbf{team\_asst} & \textbf{team\_3pt\_asst} & \textbf{player2} & \textbf{lineup\_mp} & \textbf{lineup\_poss} & \textbf{lineup\_pace} & \textbf{H/A} & \textbf{opp\_team} & \textbf{opp\_wins} & \textbf{opp\_opp\_pts} & \textbf{opp\_opp\_fg3m} \\
      2013-01-02 & 28.0 & 6 & 119 & 21 & 8 & LeBronJames & 22.4 & 47 & 99.63 & home & AL & 41 & 101.73 & 7.83 \\
2013-01-04 & 25.98 & 3 & 89 & 17 & 5 & LeBronJames & 19.2 & 32 & 82.09 & home & HI & 45 & 92.87 & 5.52 \\
2013-01-06 & 17.72 & 0 & 99 & 20 & 7 & LeBronJames & 6.4 & 11 & 74.1 & home & AS & 29 & 95.76 & 7.14 \\
2013-01-08 & 17.27 & 0 & 77 & 13 & 6 & LeBronJames & 17.3 & 31 & 115.17 & away & ND & 49 & 90.73 & 5.43 \\
2013-01-16 & 10.15 & 0 & 92 & 24 & 7 & LeBronJames & 6.3 & 12 & 87.03 & away & SW & 47 & 100.3 & 8.01 \\
2013-01-17 & 17.93 & 2 & 99 & 22 & 1 & LeBronJames & 15.2 & 28 & 103.95 & away & AL & 45 & 101.05 & 7.48 \\
2013-01-23 & 26.33 & 3 & 123 & 26 & 8 & LeBronJames & 18.1 & 32 & 83.5 & home & OR & 34 & 98.68 & 6.66 \\
2013-01-25 & 16.12 & 3 & 110 & 24 & 5 & LeBronJames & 6.8 & 11 & 82.25 & home & ET & 29 & 98.84 & 7.37 \\
 2013-01-27 & 35.98 & 2 & 98 & 19 & 4 & LeBronJames & 30.0 & 57 & 95.9 & away & OS & 41 & 96.74 & 6.79 \\
2013-01-30 & 14.0 & 3 & 105 & 21 & 8 & LeBronJames & 9.4 & 17 & 89.48 & away & KN & 49 & 95.1 & 6.32 \\
2013-02-01 & 27.8 & 11 & 89 & 21 & 4 & LeBronJames & 21.8 & 39 & 85.68 & away & ND & 49 & 90.73 & 5.43 \\
2013-02-03 & 33.72 & 5 & 100 & 19 & 2 & LeBronJames & 25.7 & 47 & 75.19 & away & OR & 34 & 98.68 & 6.66 \\
2013-02-04 & 24.17 & 5 & 99 & 23 & 1 & LeBronJames & 14.3 & 28 & 99.73 & home & HA & 21 & 102.66 & 8.73 \\
2013-02-06 & 29.13 & 12 & 114 & 23 & 9 & LeBronJames & 29.1 & 59 & 230.39 & home & OU & 45 & 102.49 & 8.06 \\
2013-02-08 & 21.03 & 12 & 111 & 22 & 12 & LeBronJames & 21.0 & 39 & 83.35 & home & AC & 56 & 94.63 & 7.65 \\
2013-02-10 & 29.18 & 9 & 107 & 19 & 5 & LeBronJames & 17.4 & 30 & 83.46 & home & AL & 45 & 101.05 & 7.48 \\
2013-02-12 & 20.63 & 9 & 117 & 22 & 7 & LeBronJames & 15.8 & 26 & 89.59 & home & OR & 33 & 100.67 & 6.35 \\
2013-02-14 & 26.83 & 6 & 110 & 23 & 8 & LeBronJames & 27.0 & 55 & 115.55 & away & KC & 60 & 96.51 & 7.44 \\
2013-02-20 & 31.8 & 17 & 103 & 23 & 9 & LeBronJames & 23.7 & 50 & 90.5 & away & TL & 44 & 97.55 & 7.56 \\
2013-02-21 & 23.18 & 3 & 86 & 20 & 3 & LeBronJames & 11.8 & 24 & 95.82 & away & HI & 45 & 92.87 & 5.52 \\
2013-02-23 & 25.13 & 6 & 114 & 27 & 9 & LeBronJames & 14.4 & 23 & 73.68 & away & HI & 34 & 96.52 & 6.7 \\
2013-02-24 & 23.77 & 14 & 109 & 23 & 11 & LeBronJames & 19.0 & 33 & 92.65 & home & LE & 24 & 101.18 & 7.44 \\
\hline
      \end{tabular}
      }
{\scriptsize
\begin{tabular}{|ccccccccccccc|} \hline
\rowcolor{grey} \textbf{player} & \textbf{year} & \textbf{month} & \textbf{avg\_mp} & \textbf{avg\_pts}  &
\textbf{avg\_team\_pts} & \textbf{avg\_team\_3ptasst} &
\textbf{avg\_mp\ w.\ LJ} &\textbf{avg\_poss\ w.\ LJ} & \textbf{avg\_pace\ w.\ LJ} & \textbf{avg\_opp\_win} & \textbf{avg\_opp\_opp\_pts} & \textbf{avg\_opp\_opp\_fg3m}  \\ \hline
$\playerSB{}$ & {\bf 2013} & {\bf 1} &  20.95 & {\bf2.20}& 101.10& 5.90  & 15.11 & 27.8 & 91.31 & 40.9	& 97.50 & 6.85\\
$\playerSB{}$ & {\bf 2013} & {\bf 2} & 26.36 & {\bf 9.08}& 104.92 &6.67& 20.08 & 37.75 & 101.30 & 40.83 &99.63 & 7.09\\
\hline
\end{tabular}
}
\end{minipage}

\begin{minipage}{0.4\linewidth}
\centering
{\footnotesize\upshape
\begin{tabular}{|ccccccc|} \hline
\rowcolor{grey} \textbf{player} & \textbf{gamedate} &\textbf{mp} &\textbf{pts} & \textbf{fgm} & \textbf{fga} & \textbf{player2}  \\ \hline
      $\playerSB{}$& 2012-11-15 & 32.52 & 18 & 6 & 7 & $\playerLJ{}$\\
      $\playerSB{}$ & 2012-11-17& 33.98 &  12 & 4 & 8 & $\playerLJ{}$ \\
      $\playerSB{}$& 2013-01-04 & 25.98 &  3 & 1 & 6 & $\playerLJ{}$ \\
      $\playerSB{}$ & 2013-01-23 & 26.33 & 3 &  1 & 3 &  $\playerLJ{}$  \\
      $\playerSB{}$  & 2013-02-06 & 29.13 & 12 &4 & 6 & $\playerLJ{}$  \\
\hline
\end{tabular}

\begin{tabular}{|ccc|} \hline
\rowcolor{grey} \textbf{mp\ w.\ p2} & \textbf{poss \ w.\ p2} & \textbf{pace \ w.\ p2} \\ \hline
 32.50 & 57 & 80.55 \\
 29.10  & 57 & 105.58\\
 19.20 & 32 & 82.09\\
 18.10 & 32 & 83.50\\
 29.10 & 59& 230.39\\
 \hline
 \end{tabular}
}
\caption{PlayerGameScoring joined with Lineup Stats}
%\vspace{-2mm}
\label{table:running-example-SBlineup}
\end{minipage}
\begin{minipage}{0.4\linewidth}
  \subfloat[\small Partial result of $Q_0$ from Example~\ref{eg:running}]{
    \begin{minipage}[b]{0.90\linewidth}\centering
    {\scriptsize
      \begin{tabular}{|cccc|} \hline
\rowcolor{grey} \textbf{player} & \textbf{year} & \textbf{month} & \textbf{avg\_pts} \\ \hline
$\playerSB{}$ & 2012 & 11 & 7.08  \\
$\playerSB{}$ & 2012 & 12 & 6.46  \\
$\playerSB{}$ & {\bf 2013} & {\bf 1} & {\bf 2.20}  \\
$\playerSB{}$ & {\bf 2013} & {\bf 2} & {\bf 9.08}  \\
$\playerSB{}$ & 2013 & 3 & 7.06  \\
\hline
\end{tabular}
}
\label{table:SB}
    \end{minipage}
  }\\
\end{minipage}

\begin{minipage}{0.4\linewidth}
\centering
\tikzset{font=\scriptsize}
\begin{tikzpicture}[
node distance=0.8cm,
longnode/.style={rectangle,draw,thin,fill=blue!20, minimum height=3mm, text width=1.8cm, align=center, on grid},
shortnode/.style={rectangle,draw,thin,fill=blue!20, minimum height=3mm, text width=0.75cm, align=center, on grid},
every loop/.style={min distance=2mm,looseness=7},
longdist/.style={distance=2cm},
shortdist/.style={distance=0.5cm}
]
  \tikzset{}
    \node[longnode]  (TGA)  {TeamGameAssist};
    \node[shortnode] (T)   [below of= TGA] {Team};
    \node[shortnode] (G)   [right=2.2cm of TGA] {Game};
    \node[longnode]  (PGS) [right=2.2cm of G]   {PlayerGameScoring};
    \node[longnode]  (LPS) [below of=G] {LineupPerGameStats};
    \node[shortnode] (L)   [below of=LPS] {Lineup};
    \node[longnode]  (LP)  [right=2.2cm of L]   {LineupPlayer};
    \node[shortnode] (P)   [below of=PGS] {Player};

  \path (TGA) edge  node[above] {$e_1$} (G)
              edge  node[left] {$e_2$} (T)
        (G)   edge  node[above] {$e_3$} (PGS)
              edge  node[left] {$e_4$} (LPS)
        (PGS) edge  node[left] {$e_5$} (P)
        (LPS) edge  node[left] {$e_6$} (L)
        (P)   edge  node[left] {$e_7$} (LP)
        (L)   edge  node[above] {$e_8$} (LP)
        (LP)  edge[loop right]  node[left] {$e_9$} (LP);
\end{tikzpicture}
\end{minipage}
\begin{minipage}{0.45\linewidth}
\centering
\tikzset{font=\footnotesize}
\begin{tikzpicture}[
  rel/.style={rectangle,draw,thin,scale=0.85,fill=blue!20},
  pred/.style={rectangle split,rectangle split parts=2, rectangle split part fill= {green!20,red!20}, draw,thin,scale=0.8,rounded corners=.8ex,text width=1.8cm,align=center},
  emph/.style={grow=down, level distance = 8mm,edge from parent/.style={black,very thick,draw}},
  norm/.style={grow=left,level distance = 20mm,sibling angle=45, edge from parent/.style={black,thin,draw}}
  ]
  \node[rel] {PT(Game)}
        child [emph]{
            node[rel] {PlayerGameScoring}
                child[norm]{node[pred]{(pts $ \geq 23)[21]$\nodepart{two} (pts$\geq 23$)$[58]$}}
                child[emph]{node[rel] {Player}
                    child[norm] {node[pred]{S.Curry \nodepart{two} S.Curry}}
                    edge from parent node [left]{$e_2$}
                    }
                edge from parent node [left]{$e_1$}
             };
\end{tikzpicture}
\end{minipage}

\begin{minipage}{0.4\linewidth}
\centering
\tikzset{font=\footnotesize}
\begin{tikzpicture}[
  rel/.style={rectangle,draw,thin,scale=0.85,fill=blue!20},
  pred/.style={rectangle split,rectangle split parts=2, rectangle split part fill= {green!20,red!20}, draw,thin,scale=0.8,rounded corners=.8ex,text width=1.5cm,align=center},
  emph/.style={level distance = 8mm,edge from parent/.style={black,very thick,draw}},
  norm/.style={level distance = 8mm , edge from parent/.style={black,thin,draw}},
  norm1/.style={grow=left, level distance = 12mm , edge from parent/.style={black,thin,draw}}
  ]
  \node[rel] {PT(Game)}
        child [emph]{
            node[rel] {LineupPerGameStats}
                % child[norm]{node[pred] {mp$\in[1,5]$ \nodepart{two} mp$\in[26,30]$ }}
                child[norm]{node[pred] {(mp$\geq 19$)$[2]$\nodepart{two}(mp$ \geq 19$)$[70]$ }}
                child[emph]{node[rel] {LineupPlayer$_1$}
                    child[emph] {node[rel]{LineupPlayer$_2$}
                        child[emph]{node[rel]{Player$_2$}
                            child[norm1]{node[pred]{G.Green \nodepart{two} G.Green}}
                            edge from parent node [left]{$e_5$}
                            }
                            edge from parent node [left]{$e_3$}
                            }
                    child[emph] {node[rel]{Player$_1$}
                        child[norm]{node[pred]{K.Thompson\nodepart{two}K.Thompson}}
                        edge from parent node [left]{$e_4$}
                        }
                        edge from parent node [left]{$e_2$}
                        }
                        edge from parent node [left]{$e_1$}
             };
\end{tikzpicture}
\end{minipage}
\begin{minipage}{0.55\linewidth}
\centering
\tikzset{font=\scriptsize}
\begin{tikzpicture}[
ns/.style={circle, draw, fill=black!50,inner sep=0.5mm},
nt/.style={}
]
\tikzset{}
    \node[ns,label=left:$g_2$] (g2)   {};
    \node[ns,label=right:$p_1$] (p1)   [right=1.8cm of g2] {};
    \node[ns,label=left:$g_3$] (g3) [below=1cm of g2]   {};
    \node[ns,label=right:$p_2$] (p2)  [below=0.3cm of p1]{};
    \node[ns,label=left:$g_5$] (g5) [below=1cm of g3] {};
    \node[ns,label=right:$p_3$] (p3)   [below=0.3cm of p2] {};
    \node[ns,label=right:$p_4$] (p4)  [below=0.3cm of p3] {};
    \node[ns,label=right:$p_5$] (p5)  [below=0.3cm of p4] {};
    \node[ns,label=right:$p_6$] (p6)  [below=0.3cm of p5] {};

    \node[nt] (game) [below=0.4cm of g5] {Game};
    \node[nt] (pgs) [below=0.45cm of p6] {PlayerGameScoring};
  \path 
      (g2)  edge[dashed]  node  {}(p1)
            edge[dashed]  node  {}(p4)
            edge[dashed]  node  {}(p6)
      (g3)  edge  node  {}(p2)
      (g5)  edge  node  {}(p3)
            edge  node  {}(p5)
      ;
\end{tikzpicture}
\end{minipage}
\caption{$\jtr(Q_1, \db, \jgraph_1)$ result using example tuples}
\label{exp:jgraph-tuple-join}
\end{figure*}

\blue{Consider $\jgraph_1$ in Figure ~\ref{Exp: curry_points}, $\jtr(Q_1, \db, \jgraph_1)$ represents the augmented provenance table. Since node is represented by \texttt{Game}, \\ $\jtr(Q_1, \db, \jgraph_1)$ here includes join results between \texttt{Game} and \\ \texttt{PlayerGameScoring} with condition as $\sglabel(\jedge_1) = (year=year \wedge month=month \wedge day=day)$. In Figure ~\ref{exp:jgraph-tuple-join}, we present the join result using the tuples from Figure ~\ref{table:game} and Figure ~\ref{table:pgs}. The dashed edges represent the result for $\jtr(Q_1, \db, \jgraph_1, t_1)$ and solid edges will be part of $\jtr(Q_1, \db, \jgraph_1, t_2)$. The tuples that are not present in \Cref{exp:jgraph-tuple-join} implies that those tuples does not join with the other relations in $\jtr(Q_1, \db, \jgraph_1)$. We will discuss in detail about how to calculate the quality measure in the next section.}

\begin{algorithm}
\caption{Generic Metaheuristic Framework}\label{Algo:meta}
{\small
	\begin{codebox}
      \Procname{SP, GP, RP, UP, TP, N( $\geq$ 1), $\mu$( $\leq$ N), $\lambda$, $\rho$ ($\leq$N)}
        \li Set iteration counter $t=0$
        \li Initialize N solutions $S_t$ randomly
        \li Evaluate each member of $S_t$
        \li Mark the best solution of $S_t$ as $x_{t}^{*}$
        \li \While{!TP}
        \li \Do
            Choose $\mu$ solutions (set $P_t$) from $S_t$ using a selection plan (SP)
            \li  Generate $\lambda$ new solutions (set $C_t$) from $P_t$ using a generation plan (GP)
            \li Choose $\rho$ solutions (set $R_t$) from $S_t$ using a replacement plan (RP)
            \li Update $S_t$ by replacing $R_t$ using $\rho$ solutions from a pool of any \\ \hspace{7mm} combination of at most three sets $P_t$, $C_t$, and $R_t$ using an update plan (UP)
            \li Evaluate each member of $S_t$
            \li Identify the best solution of $S_t$ and update $x_t^*$
            \li $t \gets t+1$
        \End
        \li Declare a near-optimal solution as $x_t^*$ 
	\end{codebox}
}
\end{algorithm}

\begin{itemize}
    \item Selection Plan(SP) : Probability $\pi_i$ of join graph $\Omega_i$ being chosen to be extended in the next iteration: $\pi_i \propto (\sigma, \phi, n, s)$
        \begin{itemize}
            \item $\sigma$: Complexity/Cost evaluating such join graph
            \item $\phi$: Recall upper bound when extending such join graph
            \item $n$: size of the join graph (number of nodes)
            \item $s$: score of the best pattern this graph generated
        \end{itemize}
    \item Generation Plan (GP): $\Omega_i'$ = Extend($\Omega_i$, rand($\bm{N},\bm{E}$))
        \begin{itemize}
            \item $\bm{N}$: set of valid nodes to be added with probabilities 
            \item $\bm{E}$: set of valid edges to be added with probabilities
        \end{itemize}
    \item Replace Plan (RP): probability of getting replaced $\gamma_i \propto \frac{1}{\pi_i}$
    \item Update Plan (UP): use new generations replace the ones selected by replace plan
    \item Terminate Plan(TP): time limit $\Delta$
\end{itemize}

\begin{algorithm}
\caption{Pattern Generation w. heuristic}\label{Algo:meta}
{\small
	\begin{codebox}
      \Procname{PatternGenerator($\bm{\Omega_0}, \lambda, \mu, k, \Delta$)}
        \li  $t=0$
        \li  $\bm{P} \gets \emptyset$
        \li  $\Lambda \gets \emptyset$
        \li \For $\omega$ in $\bm{\Omega_0}$
        \li \Do
            $P_\omega, (\omega, \sigma_\omega, \phi_\omega, n_\omega, s_\omega) \gets GenPatterns(\omega)$
            \li $\bm{P} \gets \bm{P} \cup \bm{P_\omega}$
            \li $\bm{\Lambda} \gets \bm{\Lambda} \cup (\omega, \sigma_\omega, \phi_\omega, n_\omega, s_\omega)$
            \End
        \li $\bm{\xi_k} \gets Top_k(ScoreSort(\bm{P}))$
        \li \While{$t \leq \Delta$}
        \li \Do
            $\bm{\Omega_{elite}} \gets ElitePicker(\mu, \bm{\Lambda})$ \Comment Use SP here
            \li $\bm{\Omega_{new}} \gets GraphGenerator(\bm{\Omega_{elite}},\lambda)$ \Comment Use GP here
            \li $\bm{\xi_k}, \bm{\Omega_0} \gets NaturalSelector(\bm{\Omega_{new}}, \bm{\Omega_0}, \bm{\xi_k})$ \Comment Use RP\&UP here
            \li $t \gets t+1$
            \End 
        \li \Return $\bm{\xi_k}$
	\end{codebox}
}
\end{algorithm}

% Our problem's parameters:
% \begin{itemize}
%     \item[ N]: if we generate top-K, then use K as N
%     \item[SP]: selection plan: best quality metric (F-1 + informativeness)
%     \item[GP]: generation plan: adding a node/enforcing join edge (code with probability)
%     \item[RP]: replacement plan: stratified selection: probability of getting selected is dropping from the lowest quality metric Graph to highest quality metric Graph
%     \item[UP]: Same as in Agorithm ~\ref{Algo:meta}
%     \item[TP]: terminate plan: a time limit $\Delta$
% \end{itemize}

%%% Local Variables:
%%% mode: latex
%%% TeX-master: "../main"
%%% End:
\begin{itemize}
    \item Datasets
        \begin{itemize}
            \item NBA
            \item MIMIC
            \item IMDB
            \item Synthetic for scalability?
            \item TPC-H for scalability?
        \end{itemize}
    \item Performance
        \begin{itemize}
            \item naive vs. optimization vs. existing summarization
            \item Scalability (data, attributes, queries, relations, join paths?)
        \end{itemize}
    \item Quality
        \begin{itemize}
            \item \abbrF (or final quality metric version), Precision, Recall
            \item Join vs. no join and optimized vs. naive
            \item For comparison : old explanation work
        \end{itemize}
    \item Baseline methods
        \begin{itemize}
            \item Basic Summarization
            \item Compare with ``Summarizing Provenance of Aggregation Query Results in Relational Databases'' on IMDB (for quality and scalability) and TPC-H (for scalability)
        \end{itemize}
    \item Quality (user perspective)
        \begin{itemize}
            \item User study :(
            \item Showcase concrete examples of result to convince reader
        \end{itemize}
\end{itemize}
