# Supplementary material for: Putting Things into Context: Rich Explanations for Query Answers using Join Graphs (extended version)
Source: arXiv:2103.15797 source file (2021-03-29)
Supplement: Supplementary file 2 [file appendix_experiments.tex]

\section{Appendix}

\begin{figure*}[hbt!]
    \begin{minipage}{0.495\linewidth}
    \centering
    \includegraphics[width=0.85\linewidth]{experiments/scalability_nba_new.pdf}
    \vspace{-3mm}
    \subcaption{Scalability: NBA vs different F1 sample rate}
    \label{fig:scale_nba_sample}
    \end{minipage}
    \begin{minipage}{0.495\linewidth}
        \centering
        \includegraphics[width=0.85\linewidth]{experiments/scalability_mimic_new.pdf}
        \vspace{-3mm}
        \subcaption{Scalability: MIMIC vs different F1 sample rate}
        \label{fig:scale_mimic_sample}
    \end{minipage}
    %%%%%%%%%%%%%%%%%%%%%%%%%%%%%%%%%%%%%%%%%%%%%%%%%%%%%%%%%%%%%%%%%%%%%%
    
    \begin{minipage}{0.493\linewidth}
     {
      \centering
      \scriptsize
      \begin{tabular}{|c|r|r|r|r|r|r|}
        \hline
        \textbf{db size}            & \textbf{0.1}    & \textbf{0.5}    & \textbf{1}      & \textbf{2}      & \textbf{4}       & \textbf{8}      \\
        \hline
        \textbf{feature selection} & 31.71 & 35.43 & 84.63 & 97.5 & 112.49 & 121.19 \\
        \textbf{lca} & 1.25 & 2.76 & 9.18 & 16.84 & 24.92 & 42.17 \\
        \textbf{f1 calculation} & 12.58 & 75.99 & 174.77 & 315.31 & 635.12 & 1248.13 \\
        \textbf{materialize} jg & 13.53 & 16.29 & 22 & 27.75 & 42.65 & 71.02 \\
        \textbf{refinment} & 1.98 & 10.42 & 23.25 & 46.52 & 82.08 & 176.23 \\
        \textbf{f1 sample} & 1.11 & 8.97 & 26.98 & 51.71 & 108.59 & 203.91 \\
        \hline
        \hline
        \textbf{totals} & 62.16 & 149.86 & 340.81 & 555.63 & 1005.85 & 1862.65 \\
        \hline
      \end{tabular}
      \subcaption{Scalability: Time breakdown (NBA, $\paramJoinGraphSize = 3$, f1 sample rate = 0.7)}
      \label{table:bkdown-scale-nba-sample}
    }
    \end{minipage}
     \begin{minipage}{0.493\linewidth}
     {
      \centering
      \scriptsize
      \begin{tabular}{|c|r|r|r|r|r|r|}
        \hline
        \textbf{db size}            & \textbf{0.1}    & \textbf{0.5}    & \textbf{1}      & \textbf{2}      & \textbf{4}       & \textbf{8}      \\
        \hline
        \textbf{feature selection} & 13.49 & 18.93 & 18.99 & 19.63 & 20.85 & 23.05 \\
        \textbf{lca} & 6.4 & 15.13 & 16.46 & 19.17 & 24.6 & 34.74 \\
        \textbf{f1 calculation} & 15.86 & 89.63 & 161.91 & 328.08 & 611.08 & 1133.01 \\
        \textbf{materialize jg} & 2.57 & 4.37 & 6.66 & 12.41 & 21.31 & 43.18 \\
        \textbf{refinment} & 1.67 & 8.22 & 15.49 & 32.63 & 66.84 & 133.31 \\
        \textbf{f1 sample} & 1.6 & 5.58 & 11.68 & 23.91 & 51.25 & 102.16 \\
        \hline
        \hline
        \textbf{totals} & 41.59 & 141.86 & 231.19 & 435.83 & 795.93 & 1469.45 \\
        \hline
      \end{tabular}
      \subcaption{Scalability: Time breakdown (MIMIC, $\paramJoinGraphSize = 3$, f1 sample rate = 0.7)}
      \label{table:bkdown-scale-mimic-sample}
    }
    \end{minipage}
    
     \begin{minipage}{0.493\linewidth}
      \centering
      {\scriptsize
      \begin{tabular}{|c|r|r|r|r|r|}
        \hline
        \textbf{type}           &
        \begin{minipage}{0.8cm}
          \textbf{opt: 0.1\\sample}
        \end{minipage} &
        \begin{minipage}{0.8cm}
          \textbf{opt: 0.3\\sample}
        \end{minipage}&
        \begin{minipage}{0.8cm}
          \textbf{opt: 0.5\\sample}
        \end{minipage}
        & \begin{minipage}{0.8cm}
          \textbf{opt: w/o sample}
        \end{minipage}& \textbf{naive} \\
%        \hline
        \hline
        \textbf{feature selection} & 84.96 & 87.39 & 86.86 & 84.8 & 0 \\
        \textbf{lca} & 9.43 & 9.21 & 9.25 & 9.31 & 9.39 \\
        \textbf{fscore calculation} & 33.19 & 91.5 & 149.21 & 226.53 & 16749.36 \\
        \textbf{materialize jg} & 21.96 & 21.29 & 20.87 & 20.47 & 20.51 \\
        \textbf{refinment} & 15.94 & 21.1 & 22.93 & 23.69 & 128 \\
        \textbf{f1 sample creation} & 15.52 & 21.03 & 23.44 & 0 & 0 \\
        \textbf{jg enumeration} & 17.57 & 17.76 & 17.59 & 17.43 & 17.77 \\
        \hline
        \hline
        \textbf{total} & 214.46 & 285.19 & 346.61 & 399.07 & 17017.44 \\
        \hline
      \end{tabular}
    }
          \subcaption{Naive vs Optimized: runtime breakdown in sec. (NBA, $\paramJoinGraphSize = 3$)}
      \label{table:naive_vs_opt_nba}
    \end{minipage}
    \begin{minipage}{0.493\linewidth}
      \centering
      {\scriptsize
      \begin{tabular}{|c|r|r|r|r|r|}
        \hline
        \textbf{type}           &
        \begin{minipage}{0.8cm}
          \textbf{opt: 0.1\\sample}
        \end{minipage} &
        \begin{minipage}{0.8cm}
          \textbf{opt: 0.3\\sample}
        \end{minipage}&
        \begin{minipage}{0.8cm}
          \textbf{opt: 0.5\\sample}
        \end{minipage}
        & \begin{minipage}{0.8cm}
          \textbf{opt: w/o sample}
        \end{minipage}& \textbf{naive} \\
        \hline
        \textbf{feature reduct} & 19.05 & 18.96 & 19.09 & 19.05 & 0 \\
        \textbf{lca} & 16.91 & 16.5 &  16.71 & 16.35 & 16.44 \\
        \textbf{f1 calculation} & 18.34 & 74.62 & 131.43  & 226.35  & 209.28 \\
        \textbf{materialize jg} & 6.62 &  7.08 &  6.74 &  6.65 &  6.98 \\
        \textbf{refinment} & 13.01 & 16.66 & 16.86 & 15.59 & 15.22 \\
        \textbf{f1 sample} & 6.46 &  8.8 &   9.93 &  0 &  0 \\
        \textbf{jg enumeration} & 0.24 &  0.24 &  0.24 &  0.24 &  0.24 \\
        \hline
        \hline
        \textbf{total} &  82.87 & 145.15 &   203.22 &   286.50 &   250.41 \\
        \hline
      \end{tabular}
    }
          \subcaption{Naive vs Optimized: runtime breakdown in sec. (MIMIC, $\paramJoinGraphSize = 3$)}
      \label{table:naive_vs_opt_mimic}
    \end{minipage}

\caption{Updated Experiments}
\end{figure*}
